# Supplementary material for: Insights into Alignment: Evaluating DPO and its Variants Across Multiple Tasks
Source: arXiv:2404.14723 source file (2025-02-08)
Supplement: Supplementary file 1 [file appendix_mtbench.tex]

\begin{table}[]
    \centering
    \footnotesize
    % \resizebox{\columnwidth}{!}{
    \begin{tabular}{@{}cc|ccc@{}}
        \toprule
        \thead{Model} & \thead{Align} & \thead{First Turn \\ (Score)} & \thead{Second Turn \\ (Score)} & \thead{Average \\ (Score)}
        \\
        \midrule
        Zephyr & DPO-1K & 6.81 & 6.41 & 6.61 \\
        Zephyr & DPO-5K & 7.18 & 6.71 & 6.94 \\
        Zephyr & DPO-10K & 7.12 & 6.33 & 6.72 \\
        Zephyr & DPO-61K & 7.02 & 6.48 & 6.75 \\
        \bottomrule
    \end{tabular}
    % }
    \caption{The DPO results after SFT on MT-Bench are presented for both the first and second turns. We employed the \texttt{zephyr-sft-full} model for aligning with DPO on various training sizes.}
    \label{tab:appendix_table}
\end{table}
